# Supplementary material for: Piecewise-Deterministic Optimal Path Planning
Source: arXiv:1512.08734 source file (2015-12-29)
Supplement: Supplementary file 1 [file appendixA.tex]

In section \ref{ss:Inf-Trans}, we let ${\Lambda}$ be a transition rate matrix, and $\Lambda_c = c\Lambda$ for a positive constant $c$.  Suppose $P(t)$ and $P_c(t)$ are the probability matrices corresponding to  ${\Lambda}$ and $\Lambda_c$.
In this case,
\begin{align*}
P_{c}(t)=\exp(\Lambda_{c}t)=\exp( {\Lambda}(c t)).
\end{align*}
For any initial distribution on $\M$, say, $\pi(0)$,
we have
\begin{align*}
\lim_{c\to +\infty}\pi(0)P_{c}(t) =  \lim_{c \to +\infty} \pi(0)\exp(ct{\Lambda})
= \lim_{t \to +\infty} \pi(0)P(t)
=\lim_{t\to +\infty}\pi(t).
\end{align*}

% COMMENT REMOVED
The following conclusions are proved by \textbf{Theorem 3.5.3} and \textbf{Theorem 3.6.2} in \cite{norris1998markov}:\\
For an irreducible transition rate matrix $\Lambda$ and its probability matrix $P(t)$,
\begin{itemize}
\item[(1)] There is a unique invariant distribution $\pi^*$ s.t. $\pi^*=\pi^* P(t)$ for all $t>0$;
\item[(2)] $\lim_{t\to +\infty}||\pi P(t) - \pi^*||=0$ for all initial distributions $\pi.$
\end{itemize}

Therefore,
\[\lim_{c\to +\infty}\pi(0)P_c(t) = \lim_{t\to +\infty}\pi(t) = \pi^*\]
for the invariant distribution $\pi^*$.
% COMMENT REMOVED
% COMMENT REMOVED
% COMMENT REMOVED
% COMMENT REMOVED
% COMMENT REMOVED
% COMMENT REMOVED
% COMMENT REMOVED
% COMMENT REMOVED
% COMMENT REMOVED
% COMMENT REMOVED
% COMMENT REMOVED
% COMMENT REMOVED
% COMMENT REMOVED
% COMMENT REMOVED
% COMMENT REMOVED
% COMMENT REMOVED
% COMMENT REMOVED
% COMMENT REMOVED
% COMMENT REMOVED
% COMMENT REMOVED
% COMMENT REMOVED
